# Supplementary material for: Prescribed Fire Modeling using Knowledge-Guided Machine Learning for Land Management
Source: arXiv:2310.01593 source file (2023-10-02)
Supplement: Supplementary file 1 [file appendix.tex]

The Appendix includes more details on the experimental setup, QUIC-Fire simulation setup and additional results relating to Gram-matrix loss function.

\section{Problem Setting}

\begin{figure}[ht]
    \centering
    \includegraphics[scale=0.25]{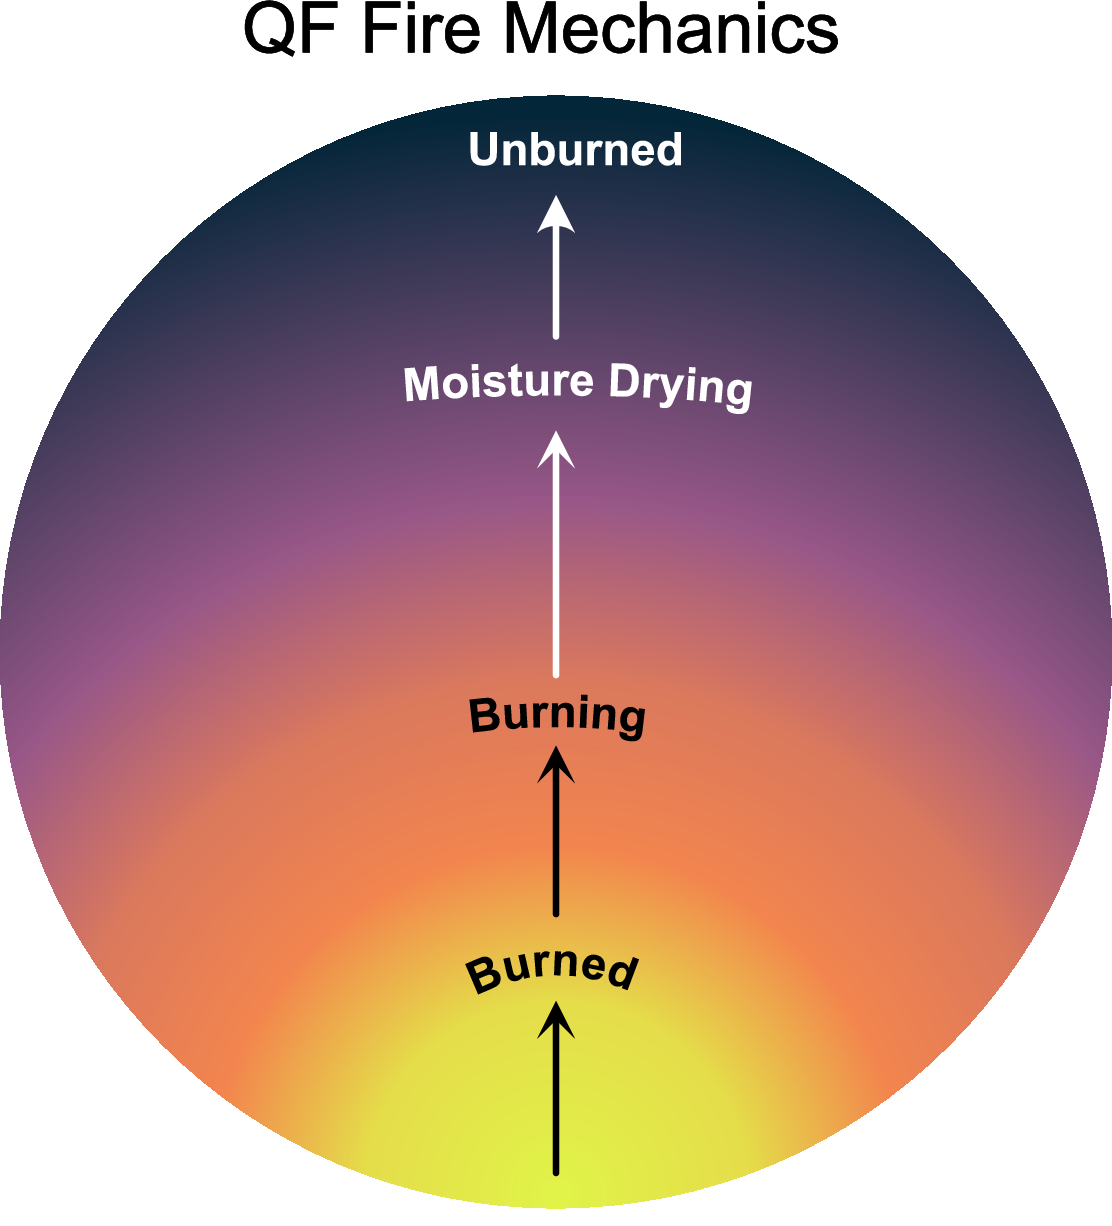}
    \caption{\small QUIC-Fire fire mechanics \cite{linn2020quic}. The fuel moisture needs to dry up before the fire starts spreading in the cell. After the moisture dries up and other conditions are met for fire ignition, the fuel burns to completion. This fire behavior further changes as other factors start influencing the mechanics. }
    \label{fig:infographic}
\end{figure}

\begin{figure}[h]
\centering
% \begin{tabular}{m{3.1cm}m{3.1cm}m{3.1cm}m{3.1cm}m{3.1cm}}
\begin{tabular}{c}
% \toprule
\centering

\subcaptionbox{\label{fig:intro} \footnotesize Ignition Pattern versus fire spread. Ignition is a precursor to spread of fire.}{\includegraphics[scale=0.17]{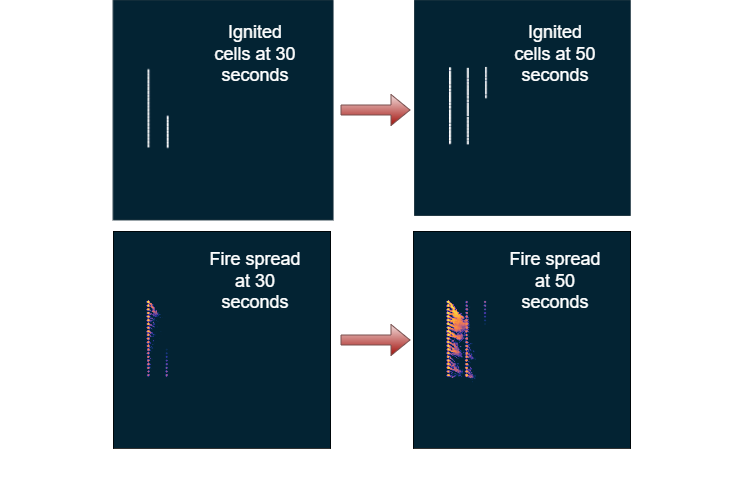}} 

\subcaptionbox{\label{fig:data_split} \footnotesize Target domain generalization.}{\includegraphics[scale=0.30]{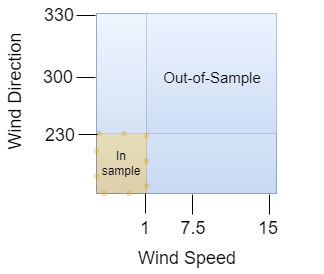}}

\end{tabular}
\caption{\small Problem Setting}
\label{fig:problem-setting}
% \vspace{-10pt}
\end{figure}

\section{More Results}

\subsection{Ablation Study}

\begin{figure*}
\centering
\includegraphics[scale=0.32]{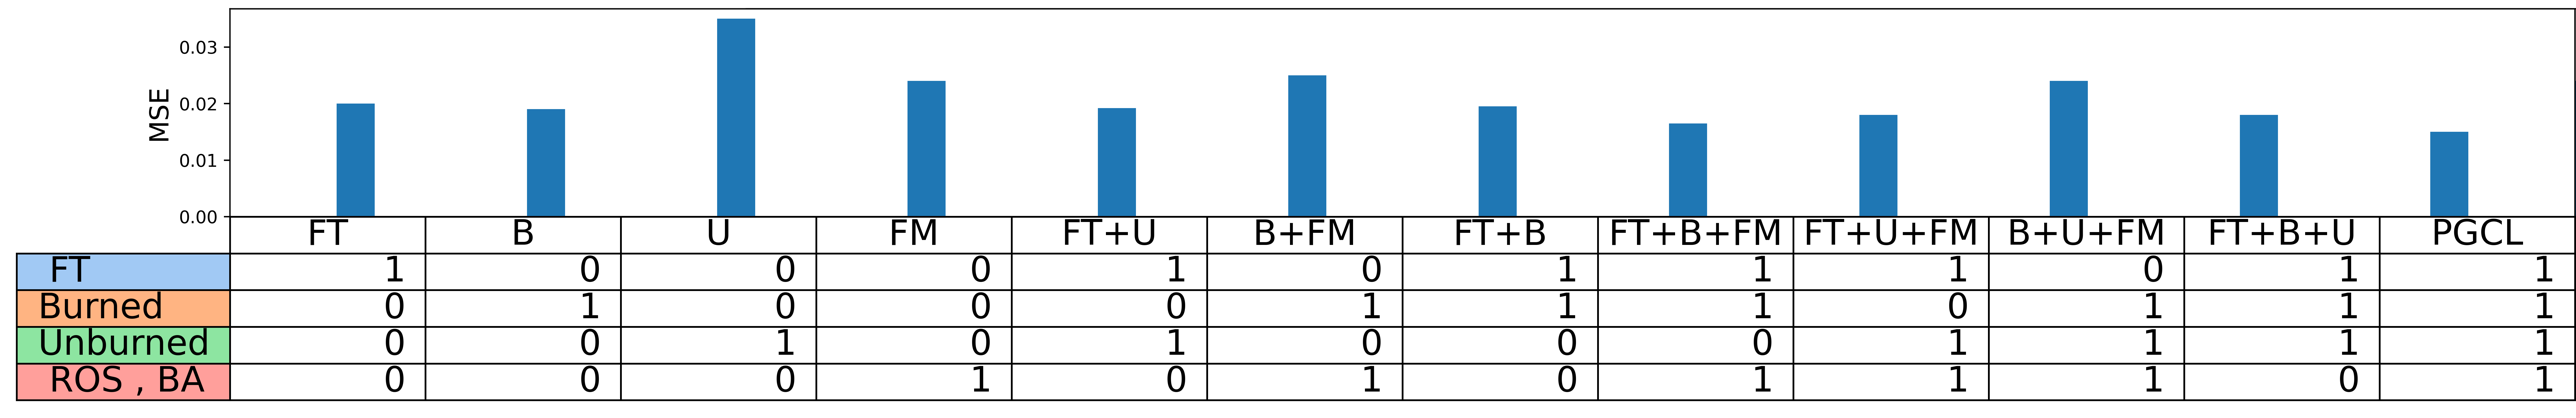}
\caption{Predictive performance varies by different physical constraints being integrated into the CL model. FT: Fuel Transport, B: Burned loss, U: Unburned loss, FM: Spread Consistency losses.}
\label{fig:ablation}
\vspace{-15pt}
\end{figure*}

Different physical constraints contribute differently in improving the model performance. In Figure~\ref{fig:ablation}, we add different physical constraints to the MSE loss function to evaluate the changes in model performance on the test set. From left to right, we add constraints (a) one-at-a-time (FT, B, U, FM), (b) two-at-a-time (FT+U, M+FM, FT+B), and then (c) three-at-a-time (FT+B+FM, FT+U+FM, B+U+FM, FT+B+U), to the base MSE loss function in the CL model. The fuel transport constraint has the most significant impact on improving the model performance. Since there is a high imbalance in the number of burned and unburned cells, regularizing burned regions specifically, helps overcome the imbalance of contribution of unburned cells in the MSE. Therefore, we see an improvement in model performance with the burned loss being added to the MSE loss function. Additionally, We see that scenario (c) has relatively lower MSEs compared to (a) and (b).

% \section{Data Setup}

% \input{problemsetting0}

\section{Baselines}

\paragraph{\textbf{CNN} \cite{cope2021using}} CNN has been used as an emulator for the QUIC-Fire model. The CNN model was the first to be able to predict burned and unburned regions with a significant reduction in computational time over QUIC-Fire. While the previously proposed CNN model forecasted the fire spread frame 50-time steps ahead, we emulate the whole fuel density sequence.

\paragraph{\textbf{CL}} We use the ConvLSTM-based spatiotemporal model proposed in the methods section as another baseline. 

\paragraph{\textbf{UNet} \cite{azad2019bi}} UNets are powerful spatiotemporal models used in a wide range of applications. We include BCDU-Net as one of the baselines. This U-Net includes Bi-directional ConvLSTM layers and reuses feature maps for precise segmentation. The densely connected convolutions enable the network to learn more diverse feature representations.

\paragraph{\textbf{FireFront} \cite{bolt2022spatio}} Firefront is a spatiotemporal autoencoder model proposed for wildfire fuel modeling. Representations are learned for inputs fire state, spatial forcing, and weather in separate encoders, passed to a UNET model to estimate the next fire state, and the decoder is used to bring the encodings back to the original fire state space. This framework was initially proposed for wildfire simulations. We modify the framework to include the input data from QUIC-Fire.

\paragraph{\textbf{CL-GL}} The CL-GL model is a further modification of the CL model with Gram loss-based regularization to match the statistical similarities between the predicted and observed fuel density.

\paragraph{\textbf{Match Baselines}} In a scenario where none of the models are available immediately for day-of planning, the historical behavior of fire can be used as an alternative to help understand future fire behavior. These historical fuel maps can be determined based on historical periods with the same initial fire conditions. We assume that the training data is available as historical fuel maps. To estimate fuel in the test set, we consider two baselines - Match ignition baseline and Match wind baseline. Match ignition baseline looks at the first fuel map in the historical data with the closest ignition pattern - while the wind conditions may vary. Match wind looks at the first fuel map in the historical data with the closest wind conditions - while the ignition pattern may vary.

\subsection{Reproducibility}

The UNet implementation can be obtained from their publicly-available repository (\href{https://github.com/rezazad68/BCDU-Net}{link}). We use Tensorflow 2.0 for building the ConvLSTM and CNN models. The code will be made publicly available.

\section{QUIC-Fire Modeling Details}

\subsection{QUIC-Fire Model Description}

QUIC-Fire is a physics-based model that represents the physical mechanisms of fire spread through a cellular automata model (Fire-CA) that is coupled with a quick diagnostic wind solver (QUIC-URB) to produce realistic representations of fire behavior and fire spread without incurring large computational expenses. QUIC-Fire is part of a suite of next generation fire behavior models that explicitly represent the relevant fuel and environmental characteristics of interest and use this detailed information to more accurately represent the complex and non-linear interactions between the evolving fire and the surrounding wind fields. This is of particular importance when modeling prescribed fires since these fire-atmospheric interactions are crucial to representing the evolution of interacting and dependent fire lines as the ignition of multiple lines whose geometry will produce plumes and indrafts that will either limit or enhance the potential spread of the surrounding fire lines. QUIC-Fire was built to run on similar inputs to full physics computational fluid dynamics (CFD) models such as FIRETEC and Wildland-Urban Fire Dynamics Simulator (WFDS), and natively runs at a horizontal resolution of 2m and vertical resolution of 1m, allowing for tight regulation of the specific allocation and arrangement of the fuels and the representation of management actions such as fire breaks and control lines. QUIC-Fire, while running significantly faster than CFD models, runs at about real-time for most simulations which is still significantly slower than what would be needed for landscape level fire response uses or even day-of test cases.

\subsection{Model and Simulation Setup}

To generate the training dataset, QUIC-Fire was run in a parameter sweep fashion for a homogeneous grassland under a variety of environmental conditions and management actions. The environmental conditions were being represented by changes in the wind speed, wind direction, and the fuel moisture across a range of what would be expected to be marginal, moderate, or extreme fire behaviour. These were chosen among the much larger set of variables that could influence fire spread in a day-of scenario such as temperature, relative humidity, atmospheric stability, etc. since they are the most easily measured and have the largest direct impact on fire spread while still responding to the larger variable set. For example, while temperature, exposure to time under sun, and relative humidity all interact and affect fire spread, they can all be in large part summarized by their effect on fuel moisture content. They are also intuitive and well understood by burn bosses who will have this information on hand when making decisions on whether the conditions are appropriate to conduct the prescribed burn. Management actions were represented by using different ignition patterns that are used in prescribed burns such as line and dot strips as well a singular ignition line, that are expected to have impact on the resulting fire characteristics. The effect of heterogeneous fuels, fuel breaks, and canopied domains which are very relevant to fire spread and the decision making in prescribed burns, will be expanded upon once the methodology for grasslands has been tested and refined.
